# Supplementary material for: Stylized Meta-Album: Group-bias injection with style transfer to study robustness against distribution shifts
Source: arXiv:2512.09773 source file (2025-12-10)
Supplement: Supplementary file 1 [file style-transfer-algorithm.tex]

\section{Neural Style Transfer algorithm}

\label{appendix:neural-style-transfer-algorithm}

For our style transfer, we used VGG-19 to reconstruct the \textit{style} and \textit{content} of input images in the following steps:
\begin{itemize}
\item First, it generates a white noise image as initialization called \textit{generated image}.
\item Then, both the \textit{content image} and the \textit{generated image} are passed through the pre-trained VGG-19 model. The squared-error content loss between the two feature representations is then defined:
\begin{equation}
L_{content} = \sum_{l=0}^L w_l \left[ \sum_{ij} (F_{ij}^l - P_{ij}^l)^2 \right]
\end{equation}

where $F^l$ is the output of \textit{content image} at layers $l$, $P^l$ is the output of \textit{generated image} at layers $l$ and $w_l$ is the weight for each layer indicating how much a layer contributes to the content loss
\item To reconstruct style, we also pass both the style image and generated image through VGG-19. The squared-error style loss between the two feature representations is then defined:
\begin{equation}
L_{style} = \sum_{l=0}^L \left[\frac{w_l}{4N_l^2M_l^2} \sum_{ij} (G_{ij}^l - A_{ij}^l)^2\right]
\end{equation}

where $A^l$ is the Gram matrix of the output of \textit{generated image} at layers $l$, $G^l$ is the Gram matrix of the output of \textit{style image} at layers $l$, $w_l$ is the weight indicating the degree to which that layer contributes to the style loss, $N_l$ is the number of channels of that layer, and $M_l$ is the total number of features - the product of the channel's height and width - for each channel of that layer.

\item Finally, we minimize the total loss function:
\begin{equation}
L_{total} = \alpha L_{content} + \beta L_{style}
\end{equation}
% with $\frac{\beta}{\alpha}=100$ and using L-BFGS as optimizer because we get the best results from these particular settings.

\begin{figure}[h]
    \centering
    \includegraphics[width=\linewidth]{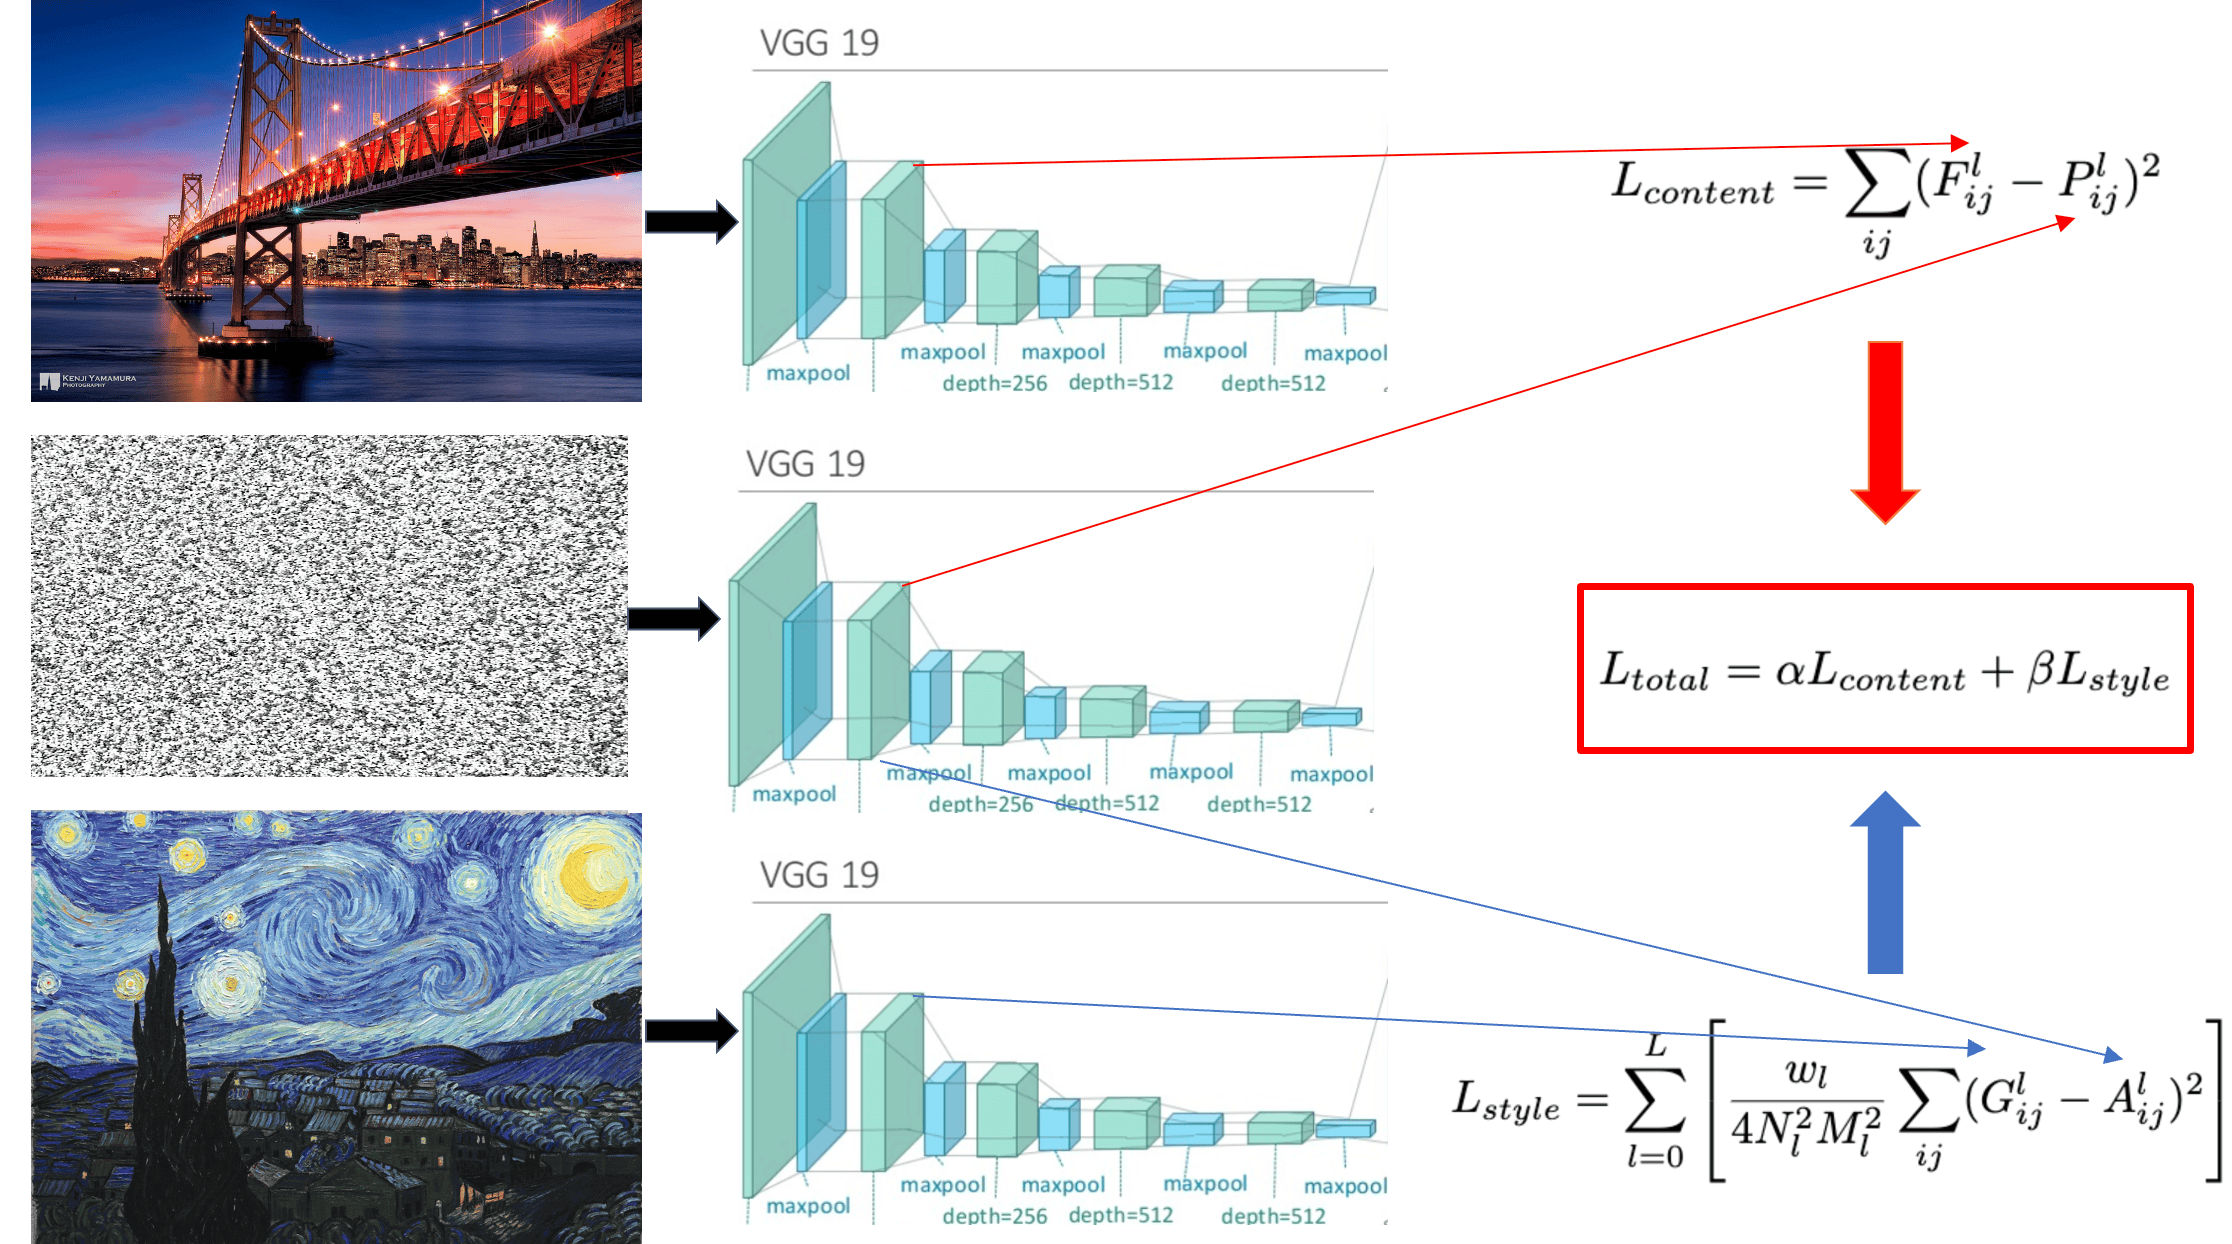}
    \caption{Style Transfer Algorithm summarization}
    \label{fig:stf-algo-summarize}
\end{figure}

\end{itemize}

By experiments, we will use the following layers to calculate the losses of Neural Style Transfer:
 conv1\_1, conv2\_1, conv3\_1, conv4\_1, and conv5.
