# Supplementary material for: Stylized Meta-Album: Group-bias injection with style transfer to study robustness against distribution shifts
Source: arXiv:2512.09773 source file (2025-12-10)
Supplement: Supplementary file 2 [file style-transfer.tex]

\section{Style Transfer}
\label{appendix:style-transfer}

We used Neural Style Transfer\cite{gatys2015neural} to introduce a different protected attribute to our dataset called \textit{style}. This \textit{style} attribute will then be used as a controlled nuisance factor Z to conduct in-depth analyses of the impact of bias in data on the generalization of several baseline methods.

Similar to the original version of Neural Style Transfer \cite{gatys2015neural}, we used VGG-19 to reconstruct the \textit{style} and \textit{content} of input images. The following parameters give the best results in our experiments:

\begin{itemize}
\item Optimizer: L-BFGS
\item Chosen layers for final loss calculation:
 conv1\_1, conv2\_1, conv3\_1, conv4\_1, and conv5
\item $\frac{\beta}{\alpha}=100$, where $\alpha$ and $\beta$ are the weights of the final loss function:
\begin{equation}
L_{total} = \alpha L_{content} + \beta L_{style}
\end{equation}
\end{itemize}
